# Supplementary material for: Quantum delocalization on correlation landscape: The key to exponentially fast multipartite entanglement generation
Source: arXiv:2404.10973 source file (2024-08-28)
Supplement: Supplementary file 1 [file supplement.pdf]

# Supplementary Materials

Yaoming Chu,[1] Xiangbei Li,[1] and Jianming Cai[1,*]

[1]*School of Physics, Hubei Key Laboratory of Gravitation and Quantum Physics, International Joint Laboratory on Quantum Sensing and Quantum Metrology, Institute for Quantum Science and Engineering, Huazhong University of Science and Technology, Wuhan 430074, China*

**Supplementary Section**

I. QFI dynamics in Krylov space

II. Exponential fast delocalization on the correlation landscape

III. Non-exponential fast delocalization on the correlation landscape

IV. Transient exponential blow-up of QFI on finite-dimensional correlation landscape

V. Full quantum analysis of atomic $SU(1,1)$ approach in Krylov space

VI. Effect of physical imperfections and decoherence

VII. Optimal interrogation operator for the entangling dynamics

**Supplementary Figures**

FIG. S1. Exponentially fast generation of global entanglement in LMG model

FIG. S2. Extended materials for Feingold-Peres model

FIG. S3. General delocalization behavior of the operator wavefunction in Krylov space

FIG. S4. Linear delocalization of the operator wavefunction in OAT model

FIG. S5. Diagonal behaviors of the correlation landscape $\mathrm{Corr}(n,m)$ in OAT model

FIG. S6. Exact QFI dynamics and saturation time in OAT model

FIG. S7. QFI dynamics and its behavior in Krylov space by $SU(1,1)$ approach

FIG. S8. Exponentially fast entanglement generation by $SU(1,1)$ approach

FIG. S9. Effect of physical imperfections of the Hamiltonian parameter in LMG model

FIG. S10. Effect of physical imperfections of the unwanted transverse field in LMG model

FIG. S11. Effect of decoherence in LMG model

FIG. S12. Correlated behaviors between the exact and approximated QFI in LMG model

## I. QFI dynamics in Krylov space

In this section, we provide a detailed derivation of QFI dynamics in the Krylov space. The Taylor expression of the time-evolved interrogation operator, $\hat{\mathcal{O}}(t) = e^{i\mathcal{L}t}\hat{\mathcal{O}} = \sum_{n=0}^{\infty}(it)^n\mathcal{L}^n\hat{\mathcal{O}}/n!$, shows that the operator dynamics can be solved in a vectorized linear space spanned by the nested commutators $\{\hat{\mathcal{O}}, \mathcal{L}\hat{\mathcal{O}}, \mathcal{L}^2\hat{\mathcal{O}}, \cdots\}$. To highlight the vector space structure, we make use of the bracket notation $|\mathcal{O})$ to regard the operator as a state in the Hilbert space of operators. Such an operator subspace can be equipped with an infinite-temperature inner product,

$$(\mathcal{O}_1|\mathcal{O}_2) := \frac{1}{\mathcal{N}}\mathrm{tr}(\hat{\mathcal{O}}_1^\dagger\hat{\mathcal{O}}_2) \tag{S.1}$$

where $\mathcal{N}$ is a constant normalization factor, for example, one can choose $\mathcal{N} = \mathrm{tr}(\hat{\mathbb{1}})$ with $\hat{\mathbb{1}}$ the identity operator of the system. Besides, we write $\|\mathcal{O}\| := (\mathcal{O}|\mathcal{O})^{1/2}$ for the norm. Based on these notations, starting from normalized vectors $|\tilde{\mathcal{O}}_0) := |\mathcal{O})/\|\mathcal{O}\|$ and $|\tilde{\mathcal{O}}_1) := \mathcal{L}|\tilde{\mathcal{O}}_0)/b_1$ with $b_1 = \|\mathcal{L}\tilde{\mathcal{O}}_0\|$, the Lanczos algorithm is defined by [1]

$$|A_n) := \mathcal{L}|\tilde{\mathcal{O}}_{n-1}) - b_{n-1}|\tilde{\mathcal{O}}_{n-2}), \quad b_n = \|A_n\|, \quad |\tilde{\mathcal{O}}_n) := |A_n)/b_n. \tag{S.2}$$

The output of this algorithm is a set of real positive Lanczos coefficients $\{b_n\}$ and the orthonormal Krylov basis $\{|\tilde{\mathcal{O}}_n)\}$, with $i^n\tilde{\mathcal{O}}_n$ being Hermitian. For simplicity, below we rescale this basis by a factor of $\|\mathcal{O}\|$, namely $\mathcal{O}_n = \|\mathcal{O}\|\tilde{\mathcal{O}}_n$. We note that the Krylov basis $\{|\mathcal{O}_n)\}$ spans the so-called Krylov space containing $\hat{\mathcal{O}}(t)$ for any evolution time $t$, but does not usually span the full space of operators. The Liouvillian superoperator is tridiagonal in this basis (i.e. $\{i^n|\mathcal{O}_n)\}$)

$$\mathcal{L} = \begin{pmatrix} 0 & ib_1 & 0 & 0 & \cdots \\ -ib_1 & 0 & ib_2 & 0 & \cdots \\ 0 & -ib_2 & 0 & ib_3 & \cdots \\ 0 & 0 & -ib_3 & 0 & \ddots \\ \vdots & \vdots & \vdots & \ddots & \ddots \end{pmatrix}. \tag{S.3}$$

Exploiting a linear expansion of the time-evolved operator in the Krylov space, i.e. $\hat{\mathcal{O}}(t) = \sum_{n=0}^{\infty} i^n\varphi_n(t)\hat{\mathcal{O}}_n$, the Heisenberg equation governed by the Liouvillian can be formulated as a discrete Schrödinger equation on a semi-infinite chain,

$$\partial_t\vec{\varphi} = i\mathcal{L}\vec{\varphi}, \quad \partial_t\varphi_n = -b_{n+1}\varphi_{n+1} + b_n\varphi_{n-1}, \quad \varphi_n(0) = \delta_{n0}, \tag{S.4}$$

where $b_0 = \varphi_{-1} = 0$ by convention.

By further taking advantage of the connection between the QFI and the time-evolved interrogation operator revealed by Eq. (1) of the main text, the QFI dynamics during the state preparation stage can be reformulated as

$$F_Q[\rho(t),\hat{\mathcal{O}}] = 4\sum_{m,n=0}^{\infty}\varphi_m(t)\varphi_n(t)\mathrm{Corr}(m,n). \tag{S.5}$$

Here, $\mathrm{Corr}(m,n)$ can be viewed as a real correlation landscape defined on Krylov basis, with an explicit formula as follows

$$\mathrm{Corr}(m,n) = \frac{\gamma}{2}\mathrm{tr}\left([i^m\hat{\mathcal{O}}_m,\sqrt{\sigma}]^\dagger[i^n\hat{\mathcal{O}}_n,\sqrt{\sigma}]\right). \tag{S.6}$$

For the special case of pure-state metrology (i.e. $\sigma = |\Psi\rangle\langle\Psi|$ represents a pure state), we have $\gamma = 1$. Thereby, the above definition recovers an explicit form of correlation function given by Eq. (4) of the main text, namely

$$\mathrm{Corr}(m,n) = \langle\hat{\mathcal{O}}_m\hat{\mathcal{O}}_n + \hat{\mathcal{O}}_n\hat{\mathcal{O}}_m\rangle/2 - \langle\hat{\mathcal{O}}_m\rangle\langle\hat{\mathcal{O}}_n\rangle. \tag{S.7}$$

Generally, the size of the Krylov basis operator gradually grows by recursive commutation with the system Hamiltonian [2]. Considering the common two-body interactions, for example, $H \sim \frac{1}{N}\sum_{\alpha\beta}J_\alpha J_\beta$ with $J_\alpha = \sum_{i=1}^N \sigma_\alpha^i$ denoting the collective spin operator and $\alpha,\beta = x,y,z$. Starting from an interrogation operator $\hat{\mathcal{O}} = J_\alpha$, the possible highest order of the Krylov basis takes the form of

$$\hat{\mathcal{O}}_{n-1} \sim \frac{1}{N^{n-1}}J_{\alpha_1}J_{\alpha_2}\cdots J_{\alpha_n} = \frac{1}{N^{n-1}}\sum_{i_1=1}^{N}\sigma_{\alpha_1}^{i_1}\sum_{i_2=1}^{N}\sigma_{\alpha_2}^{i_2}\cdots\sum_{i_n=1}^{N}\sigma_{\alpha_2}^{i_n}. \tag{S.8}$$

The correlation landscape contributed by this part is then given by

$$\begin{aligned}\mathrm{Corr}(m-1,n-1) \sim &\frac{1}{N^{m+n-2}}\sum_{i_1,i_2,\cdots,i_n,j_1,j_2,\cdots,j_m}\left[\langle\sigma_{\alpha_1}^{i_1}\sigma_{\alpha_2}^{i_2}\cdots\sigma_{\alpha_n}^{i_n}\sigma_{\beta_1}^{j_1}\sigma_{\beta_2}^{j_2}\cdots\sigma_{\beta_m}^{j_m}\rangle\right.\\ &\left.-\langle\sigma_{\alpha_1}^{i_1}\sigma_{\alpha_2}^{i_2}\cdots\sigma_{\alpha_n}^{i_n}\rangle\langle\sigma_{\beta_1}^{j_1}\sigma_{\beta_2}^{j_2}\cdots\sigma_{\beta_m}^{j_m}\rangle\right].\end{aligned} \tag{S.9}$$

We note that the number of the above summation terms equals to $N^{m+n}$, which is consistent with the fact that $\mathrm{Corr}(m,n) \lesssim N^2$ due to the normalization, e.g. $\|\hat{\mathcal{O}}_m\| = \|\hat{\mathcal{O}}_n\| = \|\hat{\mathcal{O}}\| \sim N$. In the Pauli string $\sigma_{\alpha_1}^{i_1}\sigma_{\alpha_2}^{i_2}\cdots\sigma_{\alpha_n}^{i_n}\sigma_{\beta_1}^{j_1}\sigma_{\beta_2}^{j_2}\cdots\sigma_{\beta_m}^{j_m}$, if no identical spins appears, the non-entangled feature of the initial state would lead to that

$$\langle\sigma_{\alpha_1}^{i_1}\sigma_{\alpha_2}^{i_2}\cdots\sigma_{\alpha_n}^{i_n}\sigma_{\beta_1}^{j_1}\sigma_{\beta_2}^{j_2}\cdots\sigma_{\beta_m}^{j_m}\rangle - \langle\sigma_{\alpha_1}^{i_1}\sigma_{\alpha_2}^{i_2}\cdots\sigma_{\alpha_n}^{i_n}\rangle\langle\sigma_{\beta_1}^{j_1}\sigma_{\beta_2}^{j_2}\cdots\sigma_{\beta_m}^{j_m}\rangle = 0. \tag{S.10}$$

The number of such a configuration (i.e. no identical spins appearing) is given by

$$\begin{aligned}\mathcal{N} =& N \times (N-1) \times (N-m-n+1) \\ =& N^{m+n}\left(1-\frac{1}{N}\right)\cdots\left(1-\frac{m+n-1}{N}\right) \\ \geq& N^{m+n}\left[\left(1-\frac{1}{N}\right)\left(1-\frac{m+n-1}{N}\right)\right]^{\frac{m+n}{2}} \\ \geq& N^{m+n}\left(1-\frac{m+n}{N}\right)^{\frac{m+n}{2}}\end{aligned} \tag{S.11}$$

Defining $(m+n)/2 = k$ and $(m+n)/N = \epsilon$, we can rewrite $\mathcal{N}$ as follows

$$\mathcal{N}/N^{m+n} \geq (1-\epsilon)^k = 1 - k\epsilon + C_k^2\epsilon^2 - C_k^3\epsilon^2 + \cdots \tag{S.12}$$

If $k\epsilon \ll 1, \mathcal{N} \geq N^{m+n}(1-k\epsilon)$. This result implies that the maximal number of terms that give rise to non-zero result in Eq. (S.9) is smaller than $k\epsilon N^{m+n}$, which subsequently leads to that

$$\mathrm{Corr}(m-1,n-1) \lesssim k\epsilon N^2 \simeq \frac{(m+n)^2}{N}N^2 \text{and} \quad \mathrm{Corr}(n-1,n-1) \lesssim n^2 N \tag{S.13}$$

On the contrary, $\mathrm{Corr}(n,n) \sim N^2$ would require that $k\epsilon \sim O(1)$ and thus $n \gtrsim \sqrt{N}$. This is deeply related to that the QFI achieves the Heisenberg scaling with respect to the initial product state. We point out that such a similar argument can be extended to short-range interaction as well.

## II. Exponential fast delocalization on the correlation landscape

Next, we analyze the universal delocalization properties of the 1D operator wavefunction governed by Eq. (S.4), when the Lanczos coefficients take an asymptotically linear form, i.e. $b_n = \alpha n + \gamma + o(1)$. Specifically, we employ a family of exact solutions where

$$b_n = \alpha\sqrt{n(n-1+\eta)} \quad \rightarrow \quad b_n = \alpha n + \gamma \quad \text{for} \quad n \gg 1. \tag{S.14}$$

In this case, the time-evolved operator wavefunction is analytically given by [1]

$$\varphi_n(t) = \sqrt{\frac{\Gamma(n+\eta)}{n!\Gamma(\eta)}\frac{\tanh^n(\alpha t)}{\cosh^\eta(\alpha t)}}, \tag{S.15}$$

where $\Gamma(\bullet)$ represents the Gamma function and $\Gamma(n) = (n-1)!$ for an integer $n$. As a central consequence of the linearly increased Lanczos coefficients, the operator wavefunction delocalizes in an exponentially fast speed, which can be reflected in the expected position of $\varphi_n(t)$ on the semi-infinite chain, namely

$$\mathcal{K}(t) := \sum_{n=0}^{\infty} n\varphi_n^2(t) = \eta\sinh^2(\alpha t) \sim e^{2\alpha t}. \tag{S.16}$$

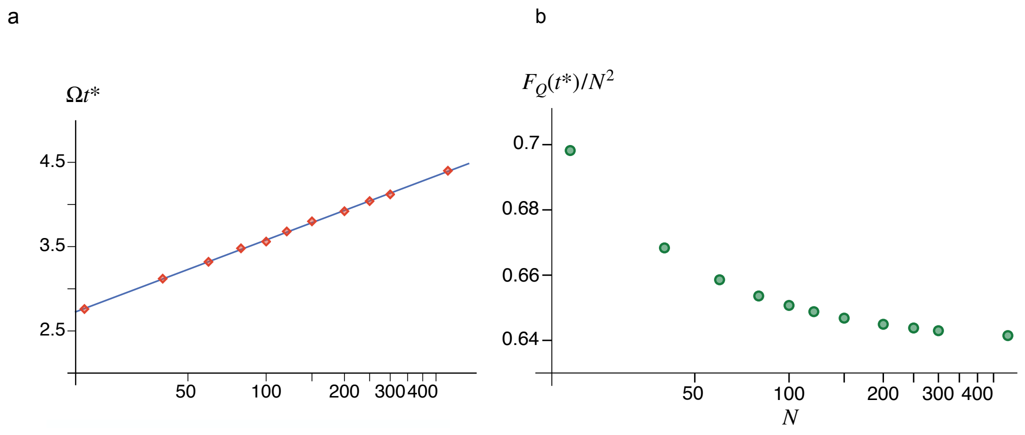


FIG. S1. **Exponentially fast generation of global entanglement in LMG model.** **(a)** The evolution time $t^*$ at which the QFI achieves its maximum shows a logarithmic relation with the system size as $\Omega t^* \approx 0.51 \log N + 1.25$. **(b)** The maximal QFI at the time $t^*$ approximately saturates to $F_Q(t^*) \approx 0.64N^2$ in the large-$N$ limit. The system parameter is set as $\chi = 2\Omega = 2$.

This quantity is also known as the Krylov complexity characterizing nonequilibrium quantum many-body dynamics, by noticing the fact that the basis operator $\hat{\mathcal{O}}_n$ becomes increasingly complex (e.g. nonlocal) with $n$.

Below, we investigate the QFI dynamics based on Eq. (S.5), by focusing on the above exponential delocalization of the operator wavefunction on the correlation landscape. Without loss of generality, we set $\eta = 1$ and utilize a simple form of the wavefunction, namely $\varphi_n(t) = \tanh^n(\alpha t)/\cosh(\alpha t)$. Consider that the correlation landscape is dominated by its diagonal stripe, and exhibits the (first local) maximum around the point $(n^*, n^*)$. Intuitively, the QFI achieves the corresponding optimum at a specific evolution time $t^*$, when the main population of the operator wavefunction approaches this point. Such a condition can be mathematically quantified by the following equation

$$p^* = \sum_{n=0}^{n^*} \varphi_n^2(t^*) = 1 - [\tanh(\alpha t^*)]^{2n^*+2}, \tag{S.17}$$

where we can roughly set $p^* = 1/2$, to indicate that the main population of $\varphi_n(t)$ reaches $n = n^*$ on the Krylov semi-infinite chain. More accurately, the deviations of the first few small Lanczos coefficients from the ideal asymptotics (i.e. $b_n = \alpha n$) might have an impact on the choice of $p^*$, by affecting the fraction of the population that can delocalize on Krylov axis. Particularly, if the first few Lanczos coefficients are relatively small as compared to the ideal ones, there might be a residual fraction of the population that always stays in the first few sites and fails to contribute

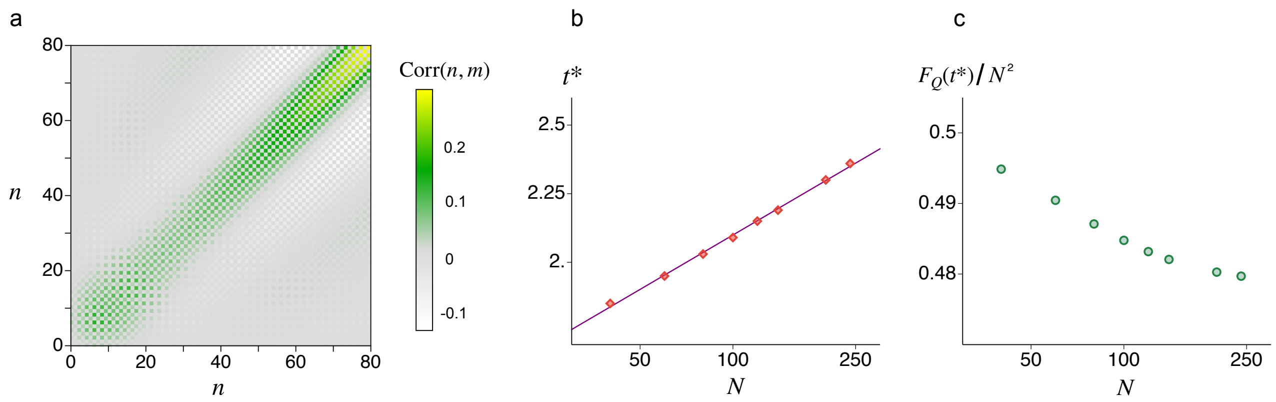


FIG. S2. **Extended materials for Feingold-Peres model.** **(a)** The correlation landscape is dominated by its diagonal stripe and exhibit the first local maximum around $(n^*, n^*) \approx (10, 10)$ for the system size $N = 80$. Combined with Fig. 3 in the main text, one can find that $n_{\rm L} \gtrsim 4n^*$ with $n_{\rm L}$ characterizing the linearly increased region of the Lanczos coefficients. This implies an exponentially fast generation of global multipartite entanglement. **(b)** The evolution time $t^*$ at which the QFI achieves its optimum shows a relation with the system size as $t^* \approx 0.29 \log N + 0.78$. **(c)** The maximal QFI at the time $t^*$ approximately saturates to $F_Q(t^*) \approx 0.48N^2$ in the large-$N$ limit. The system parameter of FP model is chosen as $c = 0$.

to the QFI growth. The most extreme case, for example, is that $b_1 = 0$ and the population would always be trapped in the initial site. In explicit scenarios, we denote the residual fraction that does not delocalize by $\mathcal{R}$, and determine the optimal evolution time $t^*$ by setting $p^* = \mathcal{R} + (1 - \mathcal{R})/2 = (1 + \mathcal{R})/2$ in Eq. (S.17).

For a finite many-body interacting system composed of $N$ particles, the linearly increased region of the Lanczos coefficients is usually up to the order of $n_{\rm L} \sim O(N)$. Before the optimal evolution time (i.e. $t = t^*$), in order to ensure an exponentially fast delocalization of the operator wavefunction—namely, $t^* \lesssim \log(N)$, we suppose that $\varphi_n(t)$ is almost fully located in the region of $[0, n_{\rm L}]$, namely

$$p^{(\rm L)} = \sum_{n=0}^{n_{\rm L}} \varphi_n^2(t^*) = 1 - [\tanh(\alpha t^*)]^{2n_{\rm L}+2} = 1 - (1 - p^*)^{(n_{\rm L}+1)/(n^*+1)} \to 1. \tag{S.18}$$

In other words, very small fraction of the population leaks out of $[0, n_{\rm L}]$, which has negligible impact on exponentially fast delocalization of the operator wavefunction. This condition can be satisfied by requiring that

$$(n_{\rm L} + 1)/(n^* + 1) \gg 1. \tag{S.19}$$

Usually, we have $n_{\rm L} \gg 1$ and $n^* \gg 1$. By setting $n_{\rm L} \geq \nu n^*$ and taking $\nu = 4$ for example, one can

obtain that $p^{(\mathrm{L})}$ is close to unit.

### III. Non-exponential fast delocalization on the correlation landscape

While focusing on the exponentially fast generation of multipartite entanglement in the main text due to its essential significance, we further discuss in this section the potential applications of our framework in non-exponential scenarios. Firstly, we study the general behaviors of operator delocalization governed by Lanczos coefficients of a generic asymptotic form $b_n = \alpha n^\delta$, i.e.

$$\partial_t \varphi_n(t) = -\alpha(n+1)^\delta \varphi_{n+1}(t) + \alpha n^\delta \varphi_{n-1}(t). \tag{S.20}$$

This differential equation, by rescaling the time parameter as $t \to \alpha t$, is equivalent to

$$\partial_t \varphi_n(t) = -(n+1)^\delta \varphi_{n+1}(t) + n^\delta \varphi_{n-1}(t). \tag{S.21}$$

Therefore, the value of the exponent $\delta$ determines universal behaviors of operator delocalization. Particularly: (i) At $\delta = 1$, exponentially fast delocalization happens and Krylov complexity grows as $\mathcal{K}(t) = \sum_n n\varphi_n(t)^2 \sim e^{2t}$. (ii) At $\delta = 1/2$ and $b_n = \sqrt{n}$, the delocalization dynamics is equivalent to a quantum harmonic oscillator starting from the vacuum state and driven by $H = i(a^\dagger - a)$, with $a$ ($a^\dagger$) the standard bosonic annihilation (creation) operator. The time-evolved state is a coherent state, namely $|\alpha\rangle = D(\alpha)|0\rangle = e^{\alpha(a^\dagger - a)}|0\rangle$ with $\alpha = t$. Using such an analogy, the Krylov

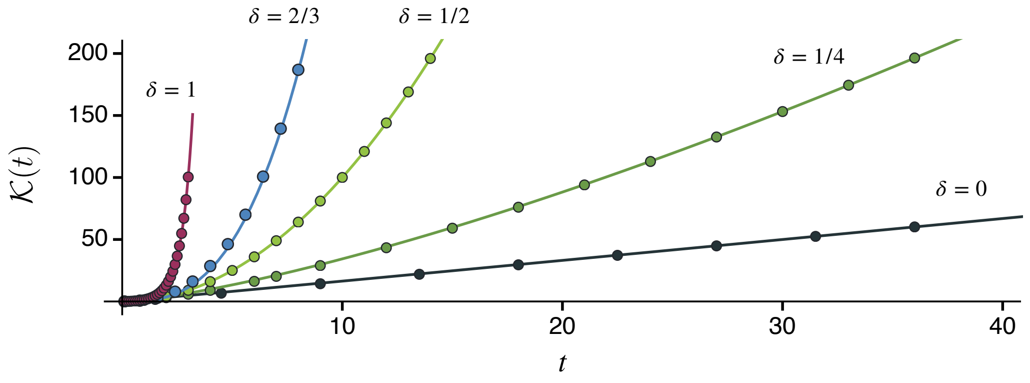


FIG. S3. **General delocalization behavior of the operator wavefunction in Krylov space.** The growth dynamics of Krylov complexity are numerically derived and then fitted for different values of the exponent $\delta$. At $\delta = 1$, the fitting yields $\mathcal{K}(t) \approx 0.23e^{2.03t}$. For $\delta < 1$, we fit the dynamics by $\mathcal{K}(t) \approx at^\xi$ with $\{a, \xi\}$ equals to $\{0.5, 2.85\}$, $\{1, 2\}$, $\{1.5, 1.36\}$ and $\{1.59, 1.01\}$ for $\delta = 2/3$, $\delta = 1/2$, $\delta = 1/4$ and $\delta = 0$ respectively.

complexity is given by the mean excitation number of the harmonic oscillator, namely $\mathcal{K}(t) = |\alpha|^2 = t^2$. (iii) At $\delta = 0$ and $b_n = 1$, the coupling between neighboring sites on the semi-infinite Krylov chain is a constant. This would lead to a linear delocalization of the operator wavefunction, i.e. $\mathcal{K}(t) \sim t$. More values of $\delta$ are illustrated in Fig. S3 by numerical fitting. Based on the numerical results, below we assume that Krylov complexity for $b_n = n^\delta$ grows as $\mathcal{K}(t) \sim t^\xi$ with the exponent $\xi$ depending on $\delta$. More specifically, we have $\xi = 1/(1-\delta)$ [2].

Similar to the proposition in the main text, if the operator wavefunction $\varphi_n(t^*)$ at the evolution time $t = t^*$, when the QFI achieves its (local) maximum, is completely covered by the asymptotic region (i.e. $b_n = n^\delta$) of the Lanczos coefficients (denoted as $[0, n_{\mathrm{L}}]$), the optimal evolution time would satisfy

$$t^* \simeq [\mathcal{K}(t^*)]^{1/\xi} \lesssim n_{\mathrm{L}}^{1/\xi} \lesssim N^{1/\xi}. \tag{S.22}$$

On the other hand, by combining with the feature of the correlation landscape, for example, $\mathrm{Corr}(n,n) \sim N^2$ requires that $n \gtrsim \sqrt{N}$, one could conjecture that a globally entangled state achieving the Heisenberg limit needs at least a generating time on the order of

$$t^* \gtrsim N^{\frac{1}{2\xi}}. \tag{S.23}$$

As an illustrative example, we consider the paradigmatic one-axis-twisting (OAT) model for en-

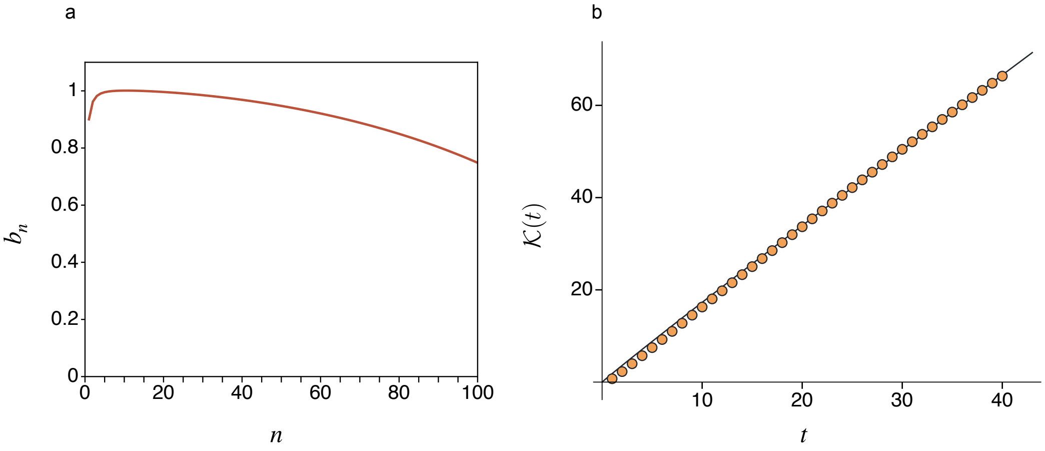


FIG. S4. **Linear delocalization of the operator wavefunction in OAT model.** **(a)** The Lanczos coefficients display no apparent growth and can be regarded as a constant. **(b)** The Krylov complexity grows linearly in time and can be well fitted by a function of $\mathcal{K}(t) \approx 1.84t^{0.97}$. Here, the system parameter is set as $\chi = 2$ and $N = 150$.

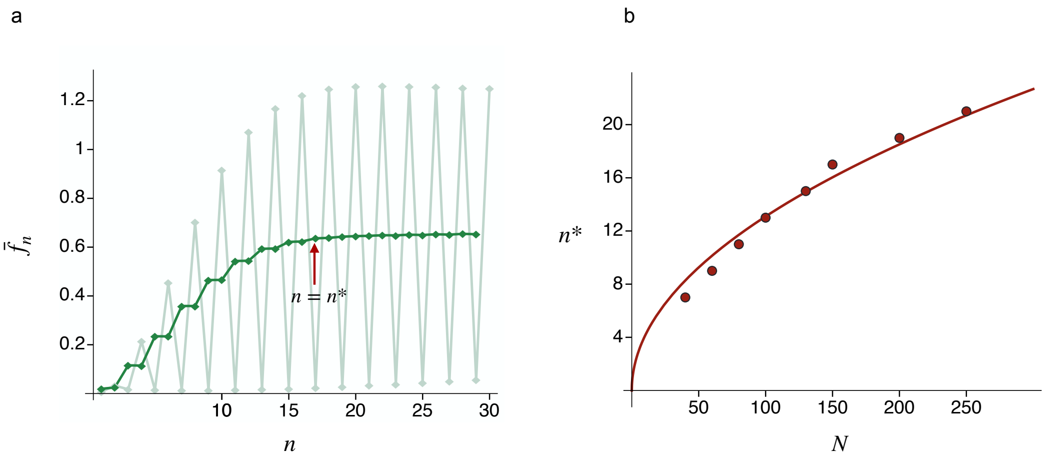


FIG. S5. **Diagonal behaviors of the correlation landscape** $\mathrm{Corr}(n, m)$ **in OAT model.** **(a)** The quantity $\bar{f}_n$ (rescaled by a factor of $N^2$) following from Eq. (9) in the main text firstly shows a linear increase and then saturates to a constant on the order of $O(1)$. Here the system size is set as $N = 150$. **(b)** The site $n^*$ where $\bar{f}_n$ starts to saturate approximately shows a square-root relation with the system size $N$, with the numerical fitting given by $n^* \approx 1.3\sqrt{N}$. The system parameter is set as $\chi = 2$.

tanglement generation [3], namely

$$\mathcal{H}_{\mathrm{OAT}} = -\frac{\chi}{N} J_x^2. \tag{S.24}$$

The initial state and interrogation operator is set as $|\Psi\rangle = |N/2\rangle = |\uparrow\uparrow\cdots\uparrow\rangle$ and $\hat{O} = J_y$ respectively. As shown in Fig. S4, the Lanczos coefficients can be approximately viewed as a constant. This results in that the operator wavefunction delocalizes linearly in Krylov space. On the other hand, we find that the correlation landscape $\mathrm{Corr}(m, n)$ is governed by its diagonal stripe. Hence, we characterize it using the quantity $\bar{f}_n$ following from Eq. (9) in the main text, which initially shows a linear increase and then starts to saturate from a certain site $n^* \approx 1.3\sqrt{N}$, as can be seen in Fig. S5. Moreover, the saturation value $\bar{f}_{n^*}$ is on the order of $O(1)$, indicating that the QFI of Heisenberg scaling (i.e. $F_Q \sim N^2$) might be achieved. Combining the above two aspects, namely the operator delocalization behavior and the feature of the correlation landscape, we conjecture that the QFI can saturate to $F_Q \simeq N^2$ from a certain time $t = t^* \sim \sqrt{N}$. This corresponds to that a global entanglement would be generated on the time scale of $t^* \sim \sqrt{N}$. We exactly verify this result in Fig. S6.

## IV. Transient exponential blow-up of QFI on finite-dimensional correlation landscape

We also apply the present general framework based on quantum delocalization on correlation

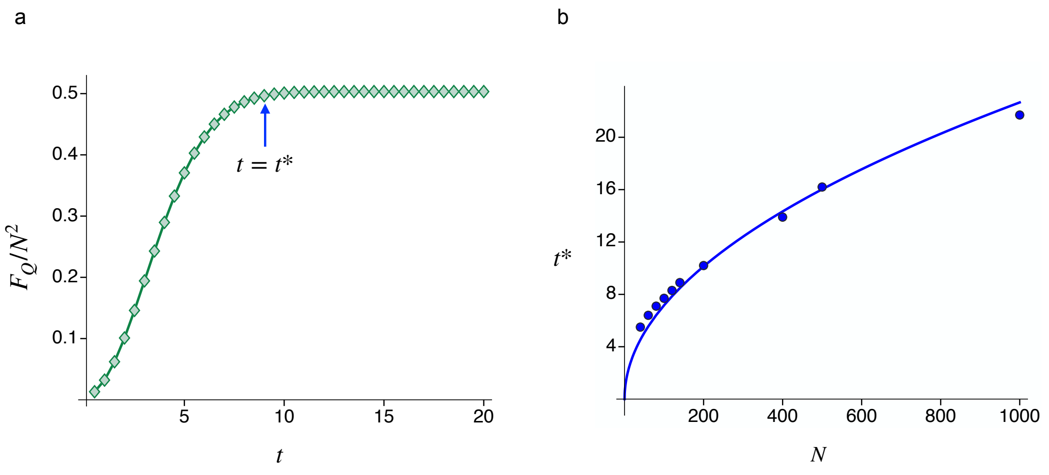


FIG. S6. **Exact QFI dynamics and saturation time in OAT model. (a)** The QFI saturates to the value of $F_Q \approx 0.5N^2$ from a certain time $t = t^*$. Here the system size is set as $N = 150$. **(b)** The saturation time $t^*$ approximately shows a square-root relation with the system size $N$, namely $t^* \approx 0.7\sqrt{N}$. The system parameter is set as $\chi = 2$.

landscape to characterize the QFI evolution where the system Hamiltonian generates a closed Lie algebra with finite dimension [4, 5]. This involves several widely-used models in the quantum information context, including the well-known inverted harmonic oscillator (IHO) [6–8] and the $SU(1,1)$ interferometric approach [9–11]. We denote a basis of the finite Lieb algebra as $\{\hat{\mathcal{O}}_0, \hat{\mathcal{O}}_1, \cdots, \hat{\mathcal{O}}_d\}$, satisfying a commutation relation $[\hat{\mathcal{O}}_n, \hat{\mathcal{O}}_m] = C_{nml}\hat{\mathcal{O}}_l$. Here, $C_{nml}$ are scalar coefficients, and the summation is performed over the repeated index. Suppose that the system Hamiltonian is a linear combination of $\{\hat{\mathcal{O}}_n\}$, namely $\mathcal{H} = \sum_n a_n \hat{\mathcal{O}}_n$ with $a_n$ being real coefficients, the Liouvillian superoperator can thus be expressed as

$$\mathcal{L} = \begin{pmatrix} \sum_n a_n C_{n00} & \sum_n a_n C_{n10} & \cdots & \sum_n a_n C_{nd0} \\ \sum_n a_n C_{n01} & \sum_n a_n C_{n11} & \cdots & \sum_n a_n C_{nd1} \\ \vdots & \vdots & \vdots & \vdots \\ \sum_n a_n C_{n0d} & \sum_n a_n C_{n1d} & \cdots & \sum_n a_n C_{ndd} \end{pmatrix}. \tag{S.25}$$

By solving the eigenvalue equation of the Liouvillian in this finite basis, namely $\mathcal{L}\hat{\Lambda}_k = \lambda_k \hat{\Lambda}_k$ , the time-evolved interrogation operator is straightforwardly given by

$$\hat{\mathcal{O}}(t) = \sum_{k=0}^{d} c_k e^{i\lambda_k t} \hat{\Lambda}_k \tag{S.26}$$

where $c_k$ are coefficients determined by the initial condition $\hat{\mathcal{O}}(0) = \hat{\mathcal{O}}$. It can be seen that if $\mathcal{L}$ has

a *negative imaginary eigenvalue*, i.e. $\mathrm{Im}(\lambda_k) < 0$ for certain $k$, the operator $\hat{\mathcal{O}}(t)$ and subsequently the QFI by using Eq. (1) in the main text would exhibit an exponential blow-up in time. In contrast, for the scenario with $C_{nml} = C^*_{nlm}$, one can directly find that $\sum_n a_n C_{nml} = \sum_n a_n C^*_{nlm}$ for arbitrary values of $\{a_n\}$, which leads to the Hermiticity and thus a real spectrum of $\mathcal{L}$, such as the celebrated $su(2)$ algebra with $C_{nml} = i\varepsilon_{nml}$ and $\varepsilon_{nml}$ denoting the Levi-Civita symbol. Consequently, the exponential blow-up of the QFI will be absent.

However, we remark that the above exponential blow-up usually holds only at short transient times, which highlights the significance of the main text focusing on the frequent infinite-dimensional scenario. The reason is that the Hamiltonian, resulting in that $\mathrm{Im}(\lambda_k) < 0$, can only describe the exact system dynamics at very initial times. For example, the IHO effectively approximates to the famous quantum Rabi model or the LMG model by requiring the condition of low bosonic excitations [12], while the atomic three-mode spin-mixing realization of $SU(1,1)$ interferometry is conditioned on the fact that a small fraction of population is transferred from the $m_f = 0$ to the $m_f = \pm 1$ hyperfine modes [13]; both conditions are satisfied only at a time scale much smaller than $\log(N)$. Below, we illustrate it using the inverted harmonic oscillator and the $SU(1,1)$ interferometry.

In the first example of the IHO, the system dynamics is governed by an inverted harmonic trapping potential, with a Hamiltonian of the following form, $H = (P^2 - \lambda X^2)/2$ and $\lambda > 0$. The IHO Hamiltonian is one of the generators of area preserving transformations, which has been widely studied as a dilatation generator, a squeezing generator, or a Lorentz boost generator, with deep connections to quantum optics, quantum Hall systems and even quantum mechanics near event horizons of black holes [14]. Up to the second order of $\{X, P\}$, one can check that the Liouvillian superoperator can be solved in a simple closed basis of $\mathcal{X} = \{\mathbb{1}, X, P, K_0, K_+, K_-\}$ with $K_0 = (XP + PX)/4$ and $K_\pm = (P^2 \pm X^2)/4$. Explicitly,

$$\mathcal{L} = \begin{pmatrix} 0 & 0 & 0 & 0 & 0 & 0 \\ 0 & 0 & -i\lambda & 0 & 0 & 0 \\ 0 & -i & 0 & 0 & 0 & 0 \\ 0 & 0 & 0 & 0 & 0 & -(1-\lambda)i \\ 0 & 0 & 0 & 0 & 0 & -(1+\lambda)i \\ 0 & 0 & 0 & 0 & (1-\lambda)i & -(1+\lambda)i \end{pmatrix}. \tag{S.27}$$

Both diagonal blocks of $\mathcal{L}$ are non-Hermitian matrices, which respectively give rise to two negative imaginary eigenvalues, $-i\sqrt{\lambda}$ and $-2i\sqrt{\lambda}$. Consequently, the quadrature operators would evolve

as $X(t) \sim \exp(\sqrt{\lambda}t)$ and $K_+ \sim \exp(2\sqrt{\lambda}t)$. This further leads to an exponential form of the QFI growth, namely

$$F_Q[\rho(t), X] \sim \exp(2\sqrt{\lambda}t) \quad \text{and} \quad F_Q[\rho(t), K_+] \sim \exp(4\sqrt{\lambda}t). \tag{S.28}$$

In quantum optics, we point out that the IHO is usually an approximate effective Hamiltonian for actual physical systems, such as the celebrated quantum Rabi model or Lipkin-Meshkov-Glick (LMG) model, by requiring the condition of low bosonic excitations in the system. More accurately, we illustrate this consition using the paradigmatic LMG example, the Hamiltonian of which reads,

$$\mathcal{H}_{\text{LMG}} = -\frac{\chi}{N}J_x^2 - \Omega J_z, \tag{S.29}$$

where $\boldsymbol{J} = (J_x, J_y, J_z)$ represents the total spin operator of the system comprised of $N$ spin-$1/2$ particles. When the system is initialized in a coherent spin state pointing along the positive $z$-axis, we can apply the Holstein-Primakoff transformation of the following form [15–17]

$$J_+ = J_x + iJ_y = \sqrt{N}\sqrt{1 - \frac{a^\dagger a}{N}}a, \tag{S.30}$$

$$J_- = J_x - iJ_y = \sqrt{N}a^\dagger\sqrt{1 - \frac{a^\dagger a}{N}} \tag{S.31}$$

$$J_z = \frac{N}{2} - a^\dagger a, \tag{S.32}$$

where $a$ ($a^\dagger$) represents the bosonic annihilation (creation) operator, obeying a standard commutation relation $[a, a^\dagger] = 1$. In the large $N$ limit—that is, within the low bosonic excitation regime (i.e. the approximation $a^\dagger a/N \ll 1$ holds), Eq. (S.46) can be approximately simplified as

$$\mathcal{H}_{\text{LMG}} = \frac{\Omega}{2}P^2 + \frac{\Omega - \chi}{2}X^2, \quad \text{with} \quad X = \frac{a + a^\dagger}{\sqrt{2}}, \quad P = \frac{a - a^\dagger}{\sqrt{2}i}. \tag{S.33}$$

By further setting that $\chi = 2\Omega > 0$, this is exactly an IHO with a maximally unstable trapping potential. The corresponding bosonic excitation of the system is given by

$$\langle a^\dagger a\rangle_t = \frac{1}{2}[\cosh(2\Omega t) - 1]. \tag{S.34}$$

This result is logically valid only when $\langle a^\dagger a\rangle_t \ll N$. Consequently, one obtains that the evolution time should satisfy a condition that $t \ll \log N/2\Omega$, in order to ensure the validity of the IHO approximation.

In the second example, we consider the $SU(1,1)$ interferometry that is described by a closed $su(1,1)$ algebra, namely

$$K_x = \frac{1}{2}(a_1^\dagger a_2^\dagger + a_1 a_2), \tag{S.35}$$

$$K_y = -\frac{i}{2}(a_1^\dagger a_2^\dagger - a_1 a_2), \tag{S.36}$$

$$K_z = \frac{1}{2}(a_1^\dagger a_1 + a_2 a_2^\dagger), \tag{S.37}$$

where $a_1$ ($a_1^\dagger$) and $a_2$ ($a_2^\dagger$) describe two bosonic modes, satisfying commutation relations $[a_i, a_j^\dagger] = \delta_{ij}$. As a result, the commutation relations for the $su(1,1)$ algebra are given by

$$[K_x, K_y] = -iK_z, \quad [K_y, K_z] = iK_x, \quad [K_z, K_x] = iK_y. \tag{S.38}$$

In atomic systems, this $SU(1,1)$ approach can be realized by exploiting a type of coherent spin-mixing dynamics in a spinor Bose-Einstein condensate. The spin-mixing dynamics describes a process of binary collisions, which can coherently transfer correlated pairs of trapped atoms from the $m_f = 0$ to the $m_f = \pm 1$ hyperfine modes with opposite magnetic moments. Explicitly, the associated many-body Hamiltonian in a dilute atomic cloud is given by [13]

$$\mathcal{H}_{\mathrm{SMD}} = \frac{\chi}{N}\left(e^{-2i\phi}a_{+1}^\dagger a_{-1}^\dagger a_0 a_0 + e^{2i\phi}a_0^\dagger a_0^\dagger a_{+1}a_{-1}\right) + \frac{\chi}{N}\left(\hat{N}_0 - \frac{1}{2}\right)(\hat{N}_{+1} + \hat{N}_{-1}) + q(\hat{N}_{+1} + \hat{N}_{-1}), \tag{S.39}$$

where $N$ is the total atom number, $\chi$ is the coupling strength of spin-mixing interaction, $q$ ($\phi$) is the energy difference (relative phase) between the $m_f = 0$ and $m_f = \pm 1$ modes, $a_i$ ($a_i^\dagger$) are bosonic annihilation (creation) operators for modes $i = m_f = 0, \pm 1$ obeying $[a_i, a_j^\dagger] = \delta_{ij}$, and $\hat{N}_i = a_i^\dagger a_i$ are the particle number operators. Experimentally, the spin-mixing process can be well controlled by microwave addressing. Theoretically, in the mean field limit—that is, the initial condensate contains a large number of particles in the $m_f = 0$ mode and the $m_f = 0$ mode operator can thus be replaced by a $c$-number, the spin-mixing operations belongs to the $SU(1,1)$ group, namely

$$\mathcal{H}_{\mathrm{SMD}} \approx 2\chi K_x + 2\tilde{q} K_z \tag{S.40}$$

where we assume $\phi = 0$ and $\tilde{q} = q + \chi(1 - 1/2N)$. As a result, the Liouvillian governing the operator dynamics is given by

$$\mathcal{L} = \begin{bmatrix} 0 & -2i\tilde{q} & 0 \\ 2i\tilde{q} & 0 & -2i\chi \\ 0 & -2i\chi & 0 \end{bmatrix}. \tag{S.41}$$

This matrix can have a negative imaginary eigenvalue, $-2i\sqrt{\chi^2-\tilde{q}^2}$, when $\chi>\tilde{q}$. Particularly, if $\tilde{q}=0$, one can obtain the operator dynamics as

$$K_z(t)=\sinh(2\chi t)K_y+\cosh(2\chi t)K_z, \tag{S.42}$$

which implies generation of a Lorentz boost amplifying the population in the $m_f=\pm1$ modes, namely

$$\langle\hat{N}_{+1}\rangle_t+\langle\hat{N}_{-1}\rangle_t=\cosh(2\chi t)-1. \tag{S.43}$$

We remark that this mean-field description is valid only when $\langle\hat{N}_{+1}\rangle_t+\langle\hat{N}_{-1}\rangle_t\ll N$, which requires that $t\ll\log N/2\chi$.

### V. Full quantum analysis of atomic $SU(1,1)$ approach in Krylov space

In this section, we perform a full three-mode quantum analysis of the Hamiltonian in Eq. (S.39) for the atomic $SU(1,1)$ interferometry. Noticing the symmetry of the system, we restrict to the Hilbert subspace spanned by Fock states $\{|N_{+1},N_0,N_{-1}\rangle=|k,N-2k,k\rangle\}$ with $0\le k\le\lfloor N/2\rfloor$. In this basis, the Hamiltonian when $N$ is even can be expressed as

$$\mathcal{H}_{\rm SMD}=\frac{\chi}{N}\begin{pmatrix}\alpha_0&\beta_0&0&0&\cdots&0\\ \beta_0&\alpha_1&\beta_1&0&\cdots&0\\ 0&\beta_1&\alpha_2&\beta_2&\cdots&0\\ 0&0&\beta_2&\alpha_3&\ddots&0\\ \vdots&\vdots&\vdots&\ddots&\ddots&\beta_{\frac{N}{2}-1}\\ 0&0&0&0&\beta_{\frac{N}{2}-1}&\alpha_{\frac{N}{2}}\end{pmatrix}+q\begin{pmatrix}0&0&0&0&\cdots&0\\ 0&2&0&0&\cdots&0\\ 0&0&4&0&\cdots&0\\ 0&0&0&6&\ddots&0\\ \vdots&\vdots&\vdots&\ddots&\ddots&0\\ 0&0&0&0&0&N\end{pmatrix}, \tag{S.44}$$

where $\alpha_k=2k(N-2k-1/2)$ and $\beta_k=(k+1)\sqrt{(N-2k)(N-2k-1)}$. We consider the conventional interrogation operator $\hat{\mathcal{O}}=(N_{+1}+N_{-1})/2$, which is given by the following matrix,

$$\hat{\mathcal{O}}=\begin{pmatrix}0&0&0&0&\cdots&0\\ 0&1&0&0&\cdots&0\\ 0&0&2&0&\cdots&0\\ 0&0&0&3&\ddots&0\\ \vdots&\vdots&\vdots&\ddots&\ddots&0\\ 0&0&0&0&0&\frac{N}{2}\end{pmatrix}, \tag{S.45}$$

the Lanczos coefficients can be numerically determined.

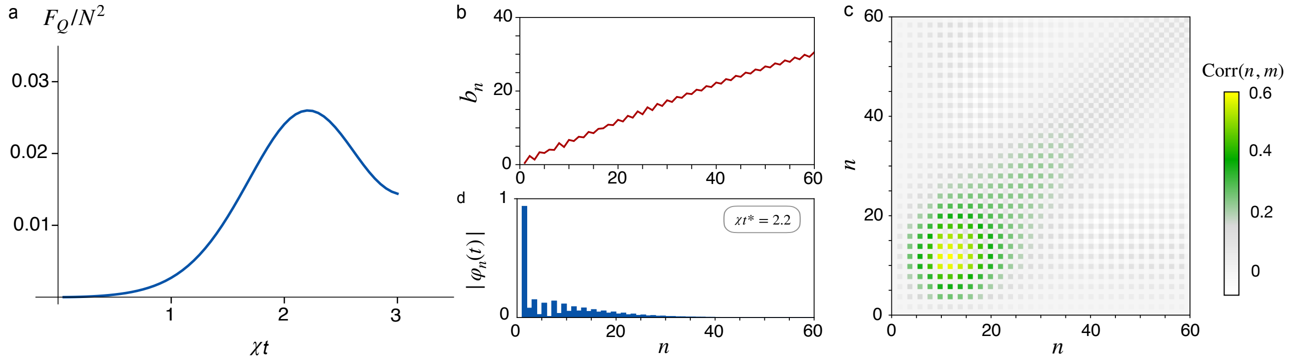


FIG. S7. **QFI dynamics and its behavior in Krylov space by $SU(1,1)$ approach.** **(a)** The QFI achieves its first local maximum around $\chi t^* = 2.2$. **(b)** The Lanczos coefficients $\{b_n\}$ show a linear increase up to the order of $n_{\rm L} \simeq N$. **(c)** The correlation landscape $\mathrm{Corr}(n, m)$ is dominated by its diagonal stripe and exhibit a local maximum around $(n^*, n^*) \approx (15, 15)$. **(d)** The fact that $n_{\rm L} \gtrsim 4n^*$ leads to that the operator wavefunction at $t^* \approx 2.2/\chi$ when the QFI is approximately optimized, is fully covered by the linearly increased region of the Lanczos coefficients, implying that the first local maximum of the QFI can be achieved exponentially fast. We choose the particle number as $N = 60$ and the system parameters as $\chi = 1$ and $q = -1$.

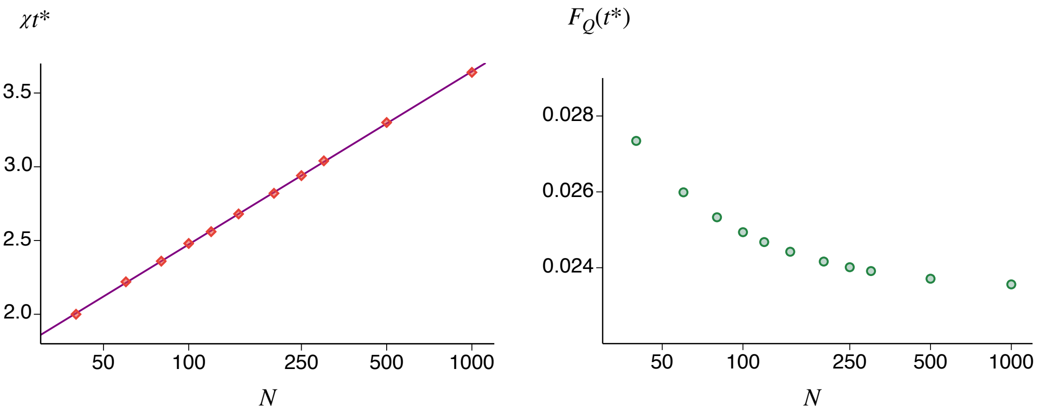


FIG. S8. **Exponentially fast entanglement generation by $SU(1,1)$ approach.** **(a)** The evolution time $t^*$ at which the QFI achieves its optimum shows a logarithmic relation with the particle number of the system, i.e. $\chi t^* \approx 0.51 \log N + 0.13$. **(b)** The maximal QFI at the time $t^*$ approximately saturates to $F_Q(t^*) \approx 0.024N^2$ in the large-$N$ limit. We set the system parameters as $\chi = 1$ and $q = -1$.

We consider the regime where the Liouvillian in Eq. (S.40) has a negative imaginary eigenvalue by setting $\chi = 1$ and $q = -1$. The corresponding numerical results in Krylov space are shown in

Fig. S7. The Lanczos coefficients show a linear increase asymptotics, and the linear region fully covers the dominant diagonal part of the correlation landscape, which indicates an exponentially fast approaching of the first local maximum of the QFI (approximately at the time $\chi t^* = 2.2$). However, one can also see that the main population of $\varphi_n(t^*)$ still stays in the first few sites, which however contribute a very small QFI. Consequently, the maximal QFI can not significantly break the standard quantum limit—that is $F_Q(t^*) \simeq \epsilon N^2$ with $\epsilon \approx 0.024 \ll 1$ (see Fig. S8).

## VI. Effect of physical imperfections and decoherence

Apart from the fundamental interest in quantum theory, creating many-particle entangled states in an exponentially fast speed is also of great importance for developing cutting-edge quantum enhanced technologies. Therefore, the physical implementation in presence of imperfections and

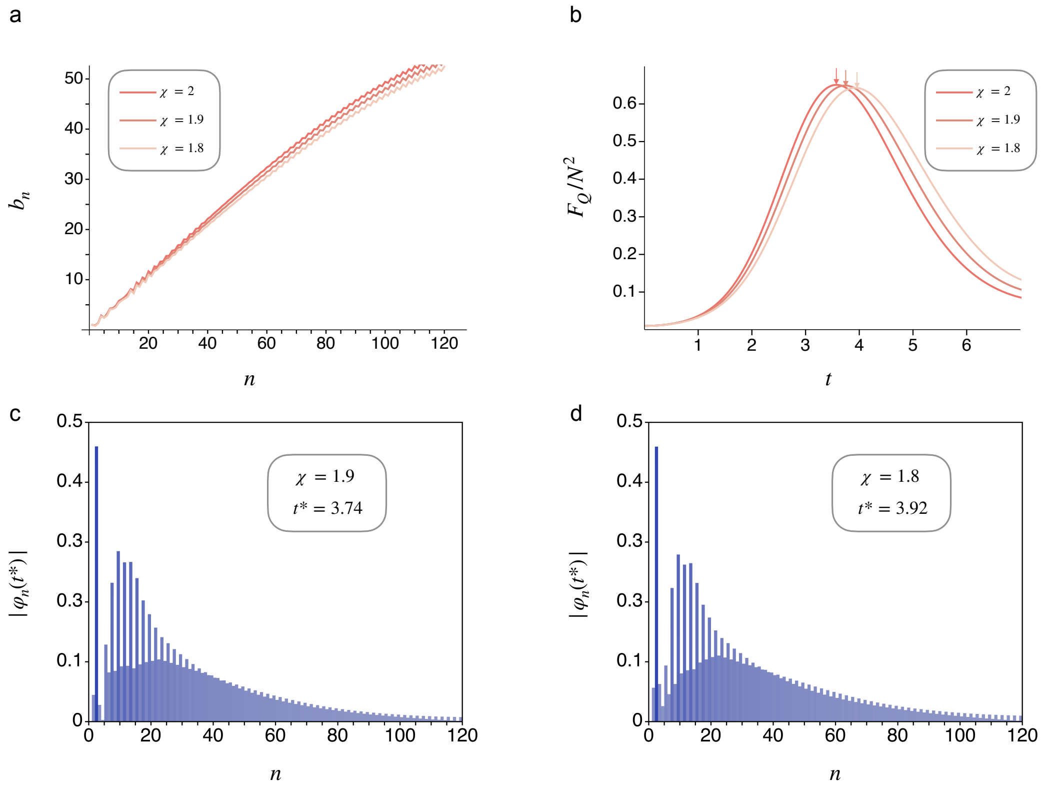


FIG. S9. **Effect of physical imperfections of the Hamiltonian parameter in LMG model. (a-b)** The Lanczos coefficients and the QFI dynamics for $\Omega = 1$ and different values of $\chi$. **(c-d)** The operator wave-functions when the QFI achieves its maximum are almost completely covered by the linear region of the Lanczos coefficients for both $\chi = 1.9$ and $\chi = 1.8$. Therefore, the exponentially fast generation of global entanglement is robust against the variation of the parameter $\chi$. Here the system size is set as $N = 100$.

decoherence in explicit quantum platforms should be carefully considered. In this section, we briefly discuss the effect of physical imperfections in implementing the entanglement generating Hamiltonian and decoherence due to interactions with the environment.

Firstly, we study the effect of physical imperfections. Considering the two examples investigated in our main text, the saddle-point dominated scrambling dynamics in the LMG model and the chaotic quantum dynamics in FP model occurs for a wide range of parameter region (i.e. $0 < \Omega < \chi/2$ and $-1 < c < 1$ respectively). This fact implies that the exponentially fast behavior of entanglement generation can be robust to variations of the system parameters. As an illustrative example, we investigate the LMG model for different values of the interaction parameter $\chi$ in Fig. S9, which demonstrates the robustness to physical imperfections of the system parameter. In

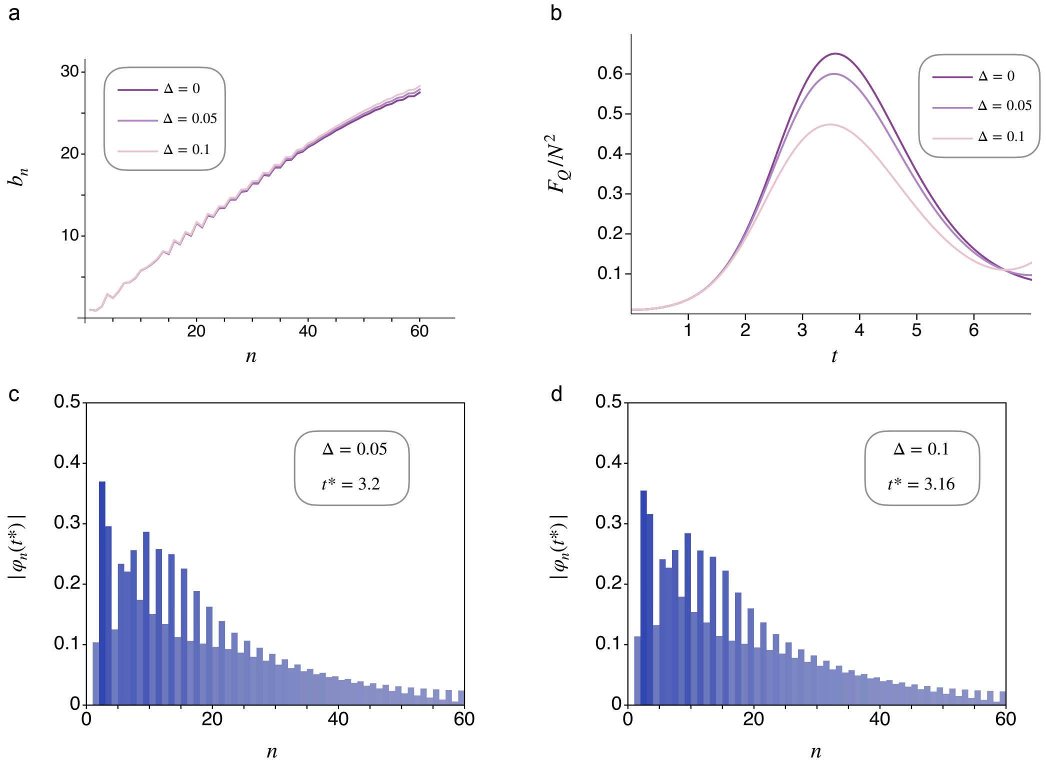


FIG. S10. **Effect of physical imperfections of the unwanted transverse field in LMG model. (a-b)** The Lanczos coefficients and the QFI dynamics for $\chi = 2\Omega = 2$ and different values of $\Delta$ in Eq. (S.46). **(c-d)** The operator wavefunctions when the QFI achieves its maximum are approximately covered by the linear region of the Lanczos coefficients for both $\Delta = 0.05$ and $\Delta = 0.1$. Therefore, the exponentially fast generation of multipartite entanglement is robust against a certain level of imperfections of the transverse field. Here the system size is set as $N = 50$.

addition, we also consider the effect of other unwanted terms when engineering the Hamiltonian, for instance, small transverse field of other directions in the LMG model,

$$\mathcal{H}'_{\mathrm{LMG}} = -\frac{\chi}{N} J_x^2 - \Omega J_z + \Delta J_x. \tag{S.46}$$

Our numerical results in Fig. S10 shows that the linear asymptotics of the Lanczos coefficients and the corresponding exponentially fast entangling dynamics can sustain with such a type of physical imperfections as well.

Secondly, we consider the effect of decoherence due to the inevitable interaction with environment. It should be pointed out that our framework based on Eq. (1) of the main text is applicable to QFI dynamics in closed systems. Currently, it is still very elusive to link QFI dynamics to the operator evolution in open quantum systems. Moreover, the Krylov approach to characterize operator delocalization, to the best of our knowledge, also merely considers the unitary dynamics governed by the system Hamiltonian, except for a very recent extension (see Ref. [18]). However, the extension assumes a Lindblad evolution of the operator to include the decoherence. Such an assumption of operator evolution cannot be simply exploited in Eq. (1) of our main text to capture the QFI dynamics. Therefore, the question how the entanglement generation speed is related to the Lanczos coefficients remains a challenging but interesting direction in the future research. Here,

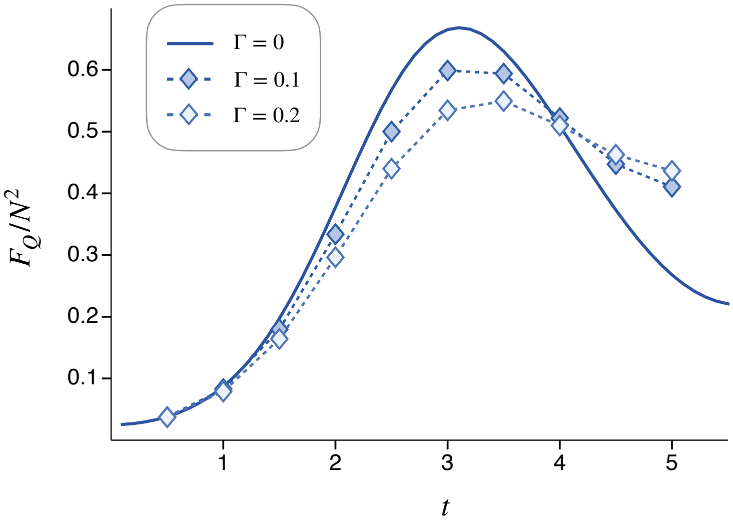


FIG. S11. **Effect of decoherence in LMG model.** We numerically derive the QFI dynamics $F_Q[\rho(t), J_x]$ for different strengths of the dephasing noises. It can be seen that the optimal time when the QFI achieves its maximum are almost the same, indicating that the exponentially fast entangling dynamics is robust to a certain level of dephasing effect. Here the system parameter is set as $\chi = 2\Omega = 2$ and $N = 40$.

we briefly study the decoherence effect by considering the LMG model through direct numerical simulation. As a simple example, we include the following dephasing noise,

$$\partial_t \rho = \mathcal{L}\rho = -i[\mathcal{H}_{\rm LMG}, \rho] + \Gamma\left(J_z \rho J_z - \frac{1}{2}\{J_z^2, \rho\}\right) \tag{S.47}$$

We solve this equation by vectorize the density operator of the system, i.e. $\rho \to |\rho\rangle\rangle$. We use the convention of the row-major vectorization, which leads the following form of the Lindblad operator governing the system dynamics

$$\mathcal{L} = -i(\mathcal{H}_{\rm LMG} \otimes \mathbb{1} - \mathbb{1} \otimes \mathcal{H}_{\rm LMG}^T) + \Gamma\left[J_z \otimes J_z^* - \frac{1}{2}\left(J_z^2 \otimes \mathbb{1} + \mathbb{1} \otimes J_z^2\right)\right]. \tag{S.48}$$

Subsequently, the time-evolved density operator is given by

$$|\rho(t)\rangle\rangle = e^{\mathcal{L}t}|\rho(0)\rangle\rangle. \tag{S.49}$$

Based on the density operator, we calculate the QFI using the following formula,

$$F_Q[\rho(t), \hat{\mathcal{O}}] = 2\gamma \mathrm{tr}([\hat{\mathcal{O}}, \sqrt{\rho(t)}]^\dagger [\hat{\mathcal{O}}, \sqrt{\rho(t)}]). \tag{S.50}$$

As one sees in Fig. S11, our straightforward numerical simulation demonstrates that the exponentially fast entanglement generation can sustain to a certain level of environmental noise.

**VII. Optimal interrogation operator for the entangling dynamics**

As one can see in Eq. (1) of the main text, the value of the QFI has close relation with the interrogation operator. For a generic multipartite interacting system, however, there is still no simple universal principles that are capable of analytically determining the optimal interrogation operator, to our best knowledge. After identifying a multipartite interacting system that enables exponentially fast generation of an entangled state $\rho$, the most straightforward way to obtain the optimal interrogation operator is optimizing the QFI value by exact numerical calculation. Given a finite-dimensional optimization set of the interrogation operator, for example, $\{O_1, O_2, \cdots, O_q\}$, we can expand the interrogation operator as $O = \sum_{\mu=1}^q \lambda_\mu O_\mu$ with $\sum_{\mu=1}^q |\lambda_\mu|^2 = 1$. Then the QFI can be re-expressed as

$$F_Q[\rho, O] = \sum_{\mu\nu} 2\gamma \lambda_\mu^* \lambda_\nu \mathrm{tr}([O_\mu, \sqrt{\rho}]^\dagger [O_\nu, \sqrt{\rho}]). \tag{S.51}$$

For pure state $\rho = |\Psi\rangle\langle\Psi|$, it further simplifies to

$$F_Q = \boldsymbol{\lambda}^T \cdot \mathcal{F} \cdot \boldsymbol{\lambda}, \tag{S.52}$$

where the vector is defined as $\boldsymbol{\lambda} = (\lambda_1, \cdots, \lambda_q)^T$, and the matrix $\mathcal{F}$ coincidentally corresponds to the quantum Fisher information matrix (QFIM) that characterizes the multi-parameter dependent state $e^{-i\sum_\mu \theta_\mu O_\mu}|\Psi\rangle$ [19]. The explicit form of QFIM component is given by

$$\mathcal{F}_{\mu\nu} = 2\langle O_\mu O_\nu + O_\nu O_\mu\rangle - 4\langle O_\mu\rangle\langle O_\nu\rangle. \tag{S.53}$$

By diagonalizing the QFIM, i.e. $F_Q = \boldsymbol{\lambda}^\dagger U^\dagger \mathcal{F}_\Lambda U \boldsymbol{\lambda}$, one can see that the largest QFI that can be achieved by the largest eigenvalue of the QFIM and the corresponding optimal interrogation operator is determined by the related eigenvector. More specifically, if $\mathcal{F}\boldsymbol{\lambda}^{(\mathrm{m})} = F^{(\max)}\boldsymbol{\lambda}^{(\mathrm{m})}$, the optimal QFI is then given by $F^{(\max)}$ and the optimal interrogation operator is

$$O^{(\mathrm{m})} = \sum_{\mu=1}^{q} \lambda_\mu^{(\mathrm{m})} O_\mu. \tag{S.54}$$

Taking the LMG model investigated in the main text as example, $|\Psi\rangle = e^{-i\mathcal{H}_{\mathrm{LMG}}t^*}|\uparrow\uparrow\cdots\uparrow\rangle$ with $t^* \approx 3.8$, the QFIM is given by

$$\mathcal{F} \approx \begin{bmatrix} 0.647 & 0.001 & 0 \\ 0.001 & 0.132 & 0 \\ 0 & 0 & 0.105 \end{bmatrix}. \tag{S.55}$$

Therefore, the optimal interrogation operator is approximately given by $O^{(\mathrm{m})} \approx J_x$, that is exactly what we considered in the main text.

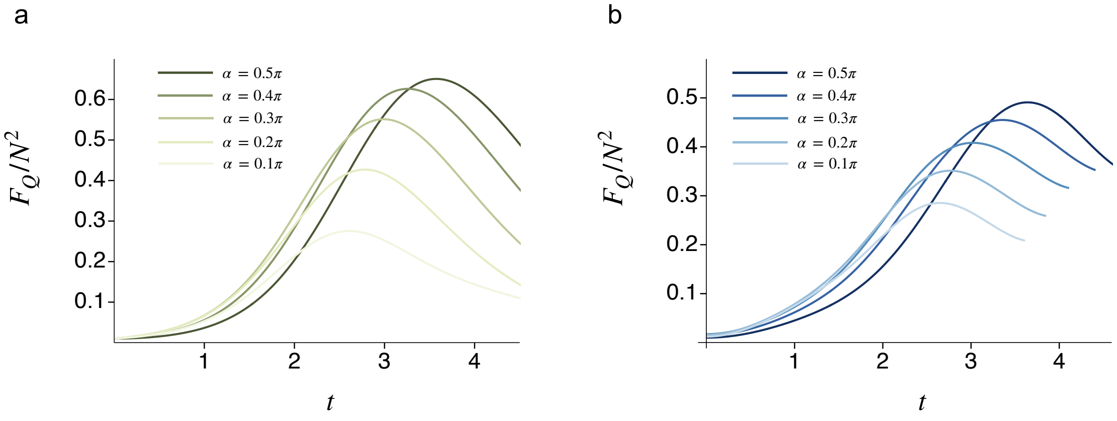


FIG. S12. **Correlated behaviors between the exact and approximated QFI in LMG model.** **(a)** The exact QFI is directly calculated for the interrogation operators $J_\alpha = \sin(\alpha)J_x + \cos(\alpha)J_y$ and achieves the maximal value at $\alpha \approx 0.5\pi$, i.e. $J_\alpha \approx J_x$. **(b)** The QFI variant, $\mathcal{F}_Q = 4\sum_n \bar{f}_n \varphi_n^2(t)$, defined by Eq. (10) in the main text, shows strongly correlated behaviors with the exact QFI dynamics. Here, the system size is set as $N = 100$ and the relevant parameters are $\chi = 2\Omega = 2$ and $w = 10$.

We also point out that the correlated behaviors between the QFI variant defined by Eq. (10) in the main text and the exact QFI might also help us to choose the interrogation operator by looking at the maximal values that the QFI variant can achieve. We illustrate this result in detail by the LMG model, as shown in Fig. S12.

---

* jianmingcai@hust.edu.cn

[1] P. Caputa, J. M. Magan, and D. Patramanis, Geometry of Krylov complexity, Phys. Rev. Res. **4**, 013041 (2022).

[2] D. E. Parker, X. Cao, A. Avdoshkin, T. Scaffidi, and E. Altman, A universal operator growth hypothesis, Phys. Rev. X **9**, 041017 (2019).

[3] L. Pezzè, A. Smerzi, M. K. Oberthaler, R. Schmied, and P. Treutlein, Quantum metrology with nonclassical states of atomic ensembles, Rev. Mod. Phys. **90**, 035005 (2018).

[4] S. Pang and T. A. Brun, Quantum metrology for a general Hamiltonian parameter, Phys. Rev. A **90**, 022117 (2014).

[5] Y. Chu, S. Zhang, B. Yu, and J. Cai, Dynamic framework for criticality-enhanced quantum sensing, Phys. Rev. Lett. **126**, 010502 (2021).

[6] C. Hotter, H. Ritsch, and K. Gietka, Combining critical and quantum metrology, Phys. Rev. Lett. **132**, 060801 (2024).

[7] K. Gietka, L. Ruks, and T. Busch, Understanding and improving critical metrology. Quenching superradiant light-matter systems beyond the critical point, Quantum **6**, 700 (2022).

[8] Z. Li, S. Colombo, C. Shu, G. Velez, S. Pilatowsky-Cameo, R. Schmied, S. Choi, M. Lukin, E. Pedrozo-Peñafiel, and V. Vuletić, Improving metrology with quantum scrambling, Science **380**, 1381 (2023).

[9] B. Yurke, S. L. McCall, and J. R. Klauder, SU(2) and SU(1,1) interferometers, Phys. Rev. A **33**, 4033 (1986).

[10] C. Gross, T. Zibold, E. Nicklas, J. Estève, and M. K. Oberthaler, Nonlinear atom interferometer surpasses classical precision limit, Nature **464**, 1165 (2010).

[11] Q. Liu, L.-N. Wu, J.-H. Cao, T.-W. Mao, X.-W. Li, S.-F. Guo, M. K. Tey, and L. You, Nonlinear interferometry beyond classical limit enabled by cyclic dynamics, Nat. Phys. **18**, 167 (2022).

[12] M.-J. Hwang, R. Puebla, and M. B. Plenio, Quantum phase transition and universal dynamics in the

Rabi model, Phys. Rev. Lett. **115**, 180404 (2015).

[13] M. Gabbrielli, L. Pezzè, and A. Smerzi, Spin-mixing interferometry with Bose-Einstein condensates, Phys. Rev. Lett. **115**, 163002 (2015).

[14] V. Subramanyan, S. S. Hegde, S. Vishveshwara, and B. Bradlyn, Physics of the inverted harmonic oscillator: From the lowest Landau level to event horizons, Ann. Phys. **435**, 168470 (2021).

[15] J. Vidal, G. Palacios, and C. Aslangul, Entanglement dynamics in the lipkin-meshkov-glick model, Phys. Rev. A **70**, 062304 (2004).

[16] S. Dusuel and J. Vidal, Finite-size scaling exponents of the lipkin-meshkov-glick model, Phys. Rev. Lett. **93**, 237204 (2004).

[17] S. Dusuel and J. Vidal, Continuous unitary transformations and finite-size scaling exponents in the lipkin-meshkov-glick model, Phys. Rev. B **71**, 224420 (2005).

[18] C. Liu, H. Tang, and H. Zhai, Krylov complexity in open quantum systems, Phys. Rev. Res. **5**, 033085 (2023).

[19] J. T. Reilly, J. D. Wilson, S. B. Jäger, C. Wilson, and M. J. Holland, Optimal generators for quantum sensing, Phys. Rev. Lett. **131**, 150802 (2023).
